# Supplementary material for: 28 GHz Phased Array-Based Self-Interference Measurements for Millimeter Wave Full-Duplex
Source: arXiv:2203.02809 source file (2022-03-05)
Supplement: Supplementary file 1 [file sec-appendix.tex]

\appendices

\section{More Plots}

\begin{figure}
	\centering
	\includegraphics[width=\linewidth,height=\textheight,keepaspectratio]{plots/full/delta_rx_per_tx-rx_beam_pair_1}
	\caption{The relative isolation of each receive beam compared to the amount of isolation achieved by a given receive beam (shown as a red $\circ$) when transmitting from the beam shown as a black $\times$.}
	\label{fig:delta-rx-per-tx-rx-beam-pair-1}
\end{figure}

\begin{figure}
	\centering
	\includegraphics[width=\linewidth,height=\textheight,keepaspectratio]{plots/full/delta_rx_per_tx-rx_beam_pair_2}
	\caption{The relative isolation of each receive beam compared to the amount of isolation achieved by a given receive beam (shown as a red $\circ$) when transmitting from the beam shown as a black $\times$.}
	\label{fig:delta-rx-per-tx-rx-beam-pair-2}
\end{figure}

\begin{figure}
	\centering
	\includegraphics[width=\linewidth,height=\textheight,keepaspectratio]{plots/full/delta_rx_per_tx-rx_beam_pair_3}
	\caption{The relative isolation of each receive beam compared to the amount of isolation achieved by a given receive beam (shown as a red $\circ$) when transmitting from the beam shown as a black $\times$.}
	\label{fig:delta-rx-per-tx-rx-beam-pair-3}
\end{figure}
